# Supplementary material for: Optical trapping and manipulation of fluorescent polymer-based nanostructures: measuring optical properties of materials in the nanoscale range
Source: arXiv:2310.04555 source file (2023-10-31)
Supplement: Supplementary file 1 [file SuppMaterial.pdf]

# Supplemental Material for “Optical trapping and manipulation of fluorescent polymer-based nanostructures: measuring optical properties of materials in the nanoscale range”

T. A. Moura<sup>1,2</sup>, M. L. Lana Júnior<sup>1</sup>, C. H. V. da Silva<sup>1</sup>, L. R. Américo<sup>1</sup>, J.

B. S. Mendes<sup>1</sup>, M. C. N. P. Brandão<sup>1</sup>, A. G. S. Subtil<sup>1</sup>, and M. S. Rocha<sup>1\*</sup>

<sup>1</sup>*Departamento de Física, Universidade Federal de Viçosa. Viçosa, Minas Gerais, Brazil. and*

<sup>2</sup>*Brazilian Nanotechnology National Laboratory (LNNano),*

*Brazilian Center for Research in Energy and Materials (CNPEM). CEP 13083-100. Campinas, São Paulo, Brazil.*

(Dated: October 31, 2023)

## I. PDOTS SYNTHESIS AND CHARACTERIZATION

Poly[2-methoxy-5-(2'-ethylhexoxy)-p-phenylene vinylene] (MEH-PPV, with an average Mn of 70-100 kDa) and tetrahydrofuran (THF- HPLC grade) were acquired from Sigma Aldrich. The pdots solution of the MEH-PPV polymer was obtained using the reprecipitation or nanoprecipitation method [1]. MEH-PPV was dissolved in THF at a concentration of 1.0 g/L and 1.0 mL of the THF solution was introduced into 10 mL of deionized water, a non-solvent, under magnetic stirring for 5 minutes. Subsequently, the solution was exposed to an ultrasonic bath for 10 minutes. The resultant solution underwent vacuum filtration using a paper filter with 2.5  $\mu\text{m}$  diameter pores. This process yields a solution containing MEH-PPV pdots.

Morphological characterization conducted using a FEG-SEM (Field Emission Gun – Scanning Electron Microscope, Tescan Mira) showed spheroid particles with diameters in the range of several hundred of nanometers, which is typical for the concentration of MEH-PPV used (Fig. 1(a)). Optical characterization (UV-Visible absorption spectra (Fig. 1(b) in the main manuscript), fluorescence spectra and anisotropy) was performed using the HORIBA Fluoromax-plusC spectrometer, placing the solution on quartz cuvettes at room temperature. The pdots solution exhibits significant fluorescence anisotropy as presented in Figure 1(b), a behavior similar to that found for MEH-PPV in solution [2]. This type of measurement was performed using established procedures [3] and agrees with the results found in OT assays, suggesting that the MEH-PPV pdots exhibit optical anisotropy.

The pdot samples for the optical tweezers experiments were prepared by filtration of the MEH-PPV pdots solution with deionized water at a volume concentration of 30%, utilizing a 0.44  $\mu\text{m}$  filter. Only the most spherical-shaped particles were selected and used in OT experiments, avoiding undesirable asymmetry effects related to particle shape.

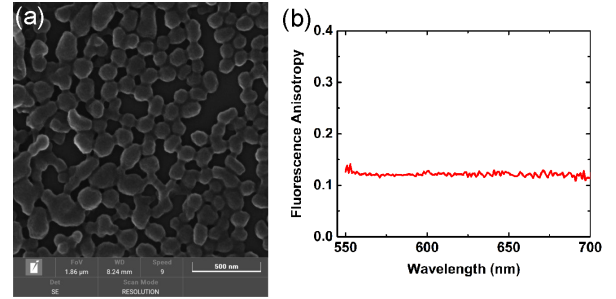

FIG. 1. (a) FEG-SEM image of a MEH-PPV pdots sample. (b) Direct fluorescence anisotropy measurement of the MEH-PPV pdots.

## II. MEASUREMENT OF THE TRAP STIFFNESS FOR THE SYSTEM OT + TRAPPED PDOTS

The transverse trap stiffness in two perpendicular directions  $\kappa_x$  and  $\kappa_y$  were measured by analyzing the Brownian position fluctuations of the trapped particles inside the optical potential well, using a standard procedure previously described in detail in ref. [4]. Basically, a CMOS camera (Basler acA1920-155uc) was used to obtain few seconds movies of each optically trapped pdot with a reliable frame rate (1,043 Hz) and a resolution of 17.1 pixel/ $\mu\text{m}$ , which allows the determination of the particle centroid with accuracy at each captured frame. The trap stiffness is then calculated from the statistics of the centroid data using the equipartition method [5]. The blur correction method of Wong and Halvorsen [6] was also employed in these analyses in order to obtain accurate results.

In Fig. 2 we show exemplifying data that illustrates the typical results obtained with our procedure. In panels (a) and (b) the histograms of the  $x$ - and  $y$ -coordinates of the centroid are shown for a  $(278 \pm 5)$  nm radius pdot. In panel (c) these coordinates are plotted simultaneously, presenting the characteristic circular distribution. Finally, panel (d) shows the mean squared displacement of a free pdot (tweezers turned off) as a function of the time, from where its radius can be determined by fitting  $\langle r^2 \rangle = 4D\Delta t$ , where  $D$  is the diffusion coefficient of the particle, given by [7]

\* marcios.rocha@ufv.br

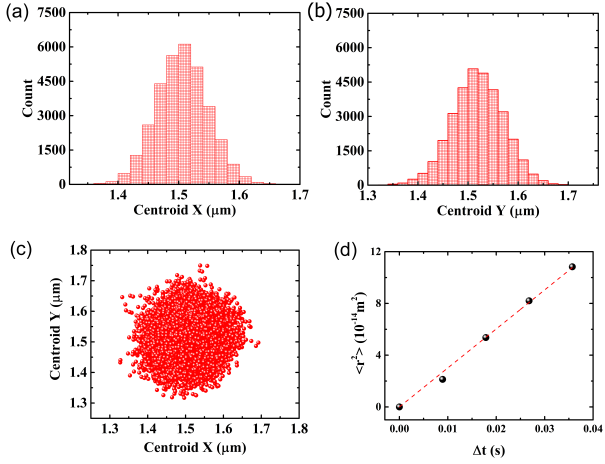

FIG. 2. (a) and (b): histograms of the  $x$ - and  $y$ -coordinates of the centroid for a  $(278 \pm 5)$  nm radius pdot. (c): coordinates plotted simultaneously, presenting the characteristic circular distribution. (d): mean squared displacement of a free pdot (tweezers turned off) as a function of the time, from where its radius can be determined.

$$D = \frac{k_B T}{6\pi\nu a \left(1 - \frac{9a}{16h} + \dots\right)^{-1}}, \quad (1)$$

where  $k_B$  is the Boltzmann's constant,  $T$  is the absolute temperature,  $\nu$  is the medium (water) viscosity,  $a$  is the particle radius and  $h$  is the particle distance from the coverslip.

Note that in this fitting all parameters are known except the particle radius, such that it can be determined with a high accuracy.

### III. A SIMPLE MODEL FOR THE OPTICAL FORCES ON THE PDOTS

When the trapped particles are much smaller than the laser wavelength employed in the tweezers, they can be treated as induced dipoles in the electric field of the laser (Rayleigh approximation). In such situation, the gradient force on the particle can be written as

$$\vec{F} = \frac{1}{2} \text{Re}(\alpha_{dyn}) \vec{\nabla} E^2, \quad (2)$$

where  $\alpha_{dyn}$  is the dynamic polarizability of the particle ( $\text{Re}$  denotes its real part) and  $\vec{E}$  is the electric field of the incident beam.

The dynamic polarizability of a spherical particle is given by [8, 9]

$$\alpha_{dyn} = 4\pi\epsilon_m \frac{\epsilon_r - 1}{\epsilon_r + 2} a^3 \left[ 1 - \frac{\epsilon_r - 1}{\epsilon_r + 2} \left( k_0^2 a^2 + \frac{2i}{3} k_0^3 a^3 \right) \right]^{-1}, \quad (3)$$

where  $\epsilon_m$  is the electric permittivity of the surrounding medium (supposed to be linear and isotropic),  $\epsilon_r$  is the relative electric permittivity of the particle to the surrounding medium,  $a$  is the particle radius and  $k_0 = 2\pi/\lambda_0$  is the wavenumber in the vacuum.

For a Gaussian ( $\text{TEM}_{00}$ ) beam the gradient of the field intensity can be straightforwardly calculated [8, 10, 11]. Using cylindrical coordinates with the  $z$ -axis coinciding with the laser propagation direction before focusing, the resulting transverse component (radial component  $\rho$ ) of the gradient force can be written as [11]

$$F_\rho = \frac{-2n}{c\epsilon_m(1+\eta)} \text{Re}(\alpha_{dyn}) \frac{\rho P}{\pi\omega^4(z)} \exp\left(\frac{-2\rho^2}{\omega^2(z)}\right) [1 - \eta \cos(2\theta)], \quad (4)$$

where  $\theta = \phi$  for  $\kappa_y$  and  $\pi/2 - \phi$  for  $\kappa_x$ ,  $n$  is the refractive index of the medium,  $c$  is the light speed in vacuum,  $P$  is the laser power at the focus,  $\omega(z)$  is the beam waist at a distance  $z$  from the focal plane [11].

The beam waist at the trapping equilibrium position was measured for our system using a camera and a calibration ruler to photograph the focused beam [4]. We found  $\omega_e = (0.99 \pm 0.09) \mu\text{m}$ , as mentioned earlier.

Since we use a linear laser polarization in our setup, an asymmetry factor  $1 - \eta \cos(2\theta)$  related to Mie resonance effects on the particle should be taken into account [11, 12], where  $\eta$  is a parameter that accounts for the relative strength of the asymmetric term [11]. The optical anisotropy of the particles, on the other hand, is related to the different values of the polarizability (and consequently of the refractive indices) returned when fitting the model to the experimental data. Such a simplified model agrees with the approach proposed by Simpson, in which the author shows that a suitable choice of the coordinate frame can lead to force equations for the anisotropic particles that are analog to the isotropic case provided that one uses the different values of the polarizability corresponding to each axis [13].

To apply the above described model to calculate the optical forces and the trap stiffness (the derivative of the force in relation to the particle position calculated at the equilibrium position), one needs to know the laser power at the focus and the radius of the trapped particle. Both quantities were directly measured in our experiments for each individual assay. The laser power at the focus was directly measured using a slide power meter designed for this purpose, as previously described [4]. The particles radius were measured by analyzing their free Brownian trajectories and calculating the diffusion coefficients as described in the former section.

- 
- [1] J. Pecher and S. Mecking, Chem. Rev. **110**, 6260 (2010).
- [2] A. J. Tilley, M. Chen, S. M. Danczak, K. P. Ghiggino, and J. M. White, Polym. Chem. **3**, 892 (2012).
- [3] Fluorecence anisotropy studies (horiba manual), <https://www.horiba.com/int/scientific/applications/biotechnology-biomedical/pages/fluorescence-anisotropy-studies/>.
- [4] U. M. S. Andrade, A. M. Garcia, and M. S. Rocha, Appl. Opt. **60**, 3422 (2021).
- [5] J. G. *et al.*, Adv. Opt. Phot. **13**, 74 (2021).
- [6] W. P. Wong and K. Halvorsen, Opt. Exp. **26**, 12517 (2006).
- [7] H. Faxen, Ann. Phys. **68**, 89 (1922).
- [8] O. M. Maragò, P. H. Jones, and G. Volpe, *Optical Tweezers: Principles and Applications*, 1st ed. (Cambridge University Press, New York, 2015).
- [9] B. T. Draine and J. Goodman, Astrophys. J. **405**, 685 (1993).
- [10] Y. Harada and T. Asakura, Opt. Commun. **124**, 529 (1996).
- [11] W. H. Campos, T. A. Moura, O. Marques, J. M. Fonseca, W. A. Moura-Melo, M. S. Rocha, and J. B. S. Mendes, Phys. Rev. Res. **1**, 033119 (2019).
- [12] R. S. Dutra, N. B. Viana, P. A. M. Neto, and H. M. Nussenzveig, J. Opt. A: Pure Appl. Opt. **9**, S221 (2007).
- [13] S. H. Simpson, J. Quant. Spec. Rad. Transf. **146**, 81 (2014).
